# Supplementary material for: Dense scale selection over space, time and space-time
Source: arXiv:1709.08603 source file (2018-08-03)
Supplement: Supplementary file 1 [file Index_supplementary_materials-rev1.pdf]

**Index of Supplementary Materials**

Title of paper: *Dense scale selection over space, time and space-time*
Authors: *Tony Lindeberg*

File: supplement-rev1.pdf
Type: PDF file with text
Contents: The supplement provides complementary details that could not be included in the main paper because of space limitations.
Justification: Supplement SM1 shows how the selected spatial scales can be analysed in the presence of post-smoothing. Supplement SM2 shows how phase compensation can be performed in the spatio-temporal case and describes more details regarding the influence of the parameters Gamma_s and Gamma_tau.

Files:

```
smoothwaves_effspatscale.mp4
smoothwaves_efftempscale.mp4
smoothwaves_grey.mp4
smoothwaves_maxmagn.mp4
smoothwaves_quasi.mp4
smoothwaves_scspsign.mp4

smoothtraffic_effspatscale.mp4
smoothtraffic_efftempscale.mp4
smoothtraffic_grey.mp4
smoothtraffic_maxmagn.mp4
smoothtraffic_quasi.mp4
smoothtraffic_scspsign.mp4

breakingwaves_effspatscale.mp4
breakingwaves_efftempscale.mp4
breakingwaves_grey.mp4
breakingwaves_maxmagn.mp4
breakingwaves_quasi.mp4
breakingwaves_scspsign.mp4
```

Type: MPEG-4 videos with experimental results

Contents:

The files with prefix ”smoothwaves” show videos with the experimental results shown as snapshots in Figure 8.

The files with prefix ”smoothtraffic” show videos with the experimental results shown as snapshots in Figure 9.

The files with prefix ”breakingwaves” show videos with the experimental results shown as snapshots in Figure 10.

The files with suffix ”grey”, show the original grey-level video (as shown in the upper left of each figure).

The files with suffix ”quasi”, show the the quasi quadrature measure at a fixed scale (as shown in the upper right of each figure).

The files with suffix ”effspatscale”, show the selected spatial scales in units of effective scale (as shown in the middle left of each figure).

The files with suffix ”efftempscale”, show the selected temporal scales in units of effective scale (as shown in the middle right of each figure).

The files with suffix ”scspsign”, show the scale-space signature (as shown in the bottom left of each figure).

The files with suffix ”maxmagn”, show the maximum magnitude response over all spatio-temporal scales (as shown in the bottom right of each figure).

Justification: Reviewer 1 asked for videos of the results for Figures 8-9. I do also enclose corresponding results also for Figure 10, for completeness and consistency (or if the restriction to just two of these three figures of similar type could have been a typing error).

These videos make it much easier for the reader to understand the dynamics of the video results, which cannot be visualized in print.
